# Supplementary material for: X-Risk Analysis for AI Research
Source: arXiv:2206.05862 source file (2022-09-20)
Supplement: Supplementary file 1 [file kill_supp.tex]

\documentclass{article}

\usepackage[nonatbib]{neurips_data_2021}
\usepackage[round,semicolon]{natbib}

\usepackage[utf8]{inputenc} %
\usepackage[T1]{fontenc}    %
\usepackage{hyperref}       %
\usepackage{url}            %
\usepackage{booktabs}       %
\usepackage{amsfonts}       %
\usepackage{nicefrac}       %
\usepackage{microtype}      %
\usepackage{xcolor}         %

\input{math_commands.tex}

\usepackage{hyperref}
\usepackage{url}
\usepackage{lipsum}
\usepackage{bbm}
\usepackage{booktabs}
\usepackage{tabularx}
\newcolumntype{Y}{>{\centering\arraybackslash}X}
\newcolumntype{s}{>{\hsize=.3\hsize}Y}
\newcolumntype{t}{>{\hsize=.7\hsize}X}
\newcolumntype{b}{X}
\newcolumntype{u}{>{\hsize=0.8\hsize}Y}
\usepackage{multirow}
\usepackage{makecell}
\usepackage{wrapfig}
\usepackage{graphicx}
\usepackage{enumitem}
\usepackage{subcaption}
\hypersetup{
    colorlinks=true,
	linkcolor=blue,
	filecolor=magenta,      
	urlcolor=blue,
	citecolor=black,
	pdfinfo={
		Title={What Would Jiminy Cricket Do? Towards Agents That Behave Morally},
		Author={Dan Hendrycks, Mantas Mazeika, Andy Zou, Sahil Patel, Christine Zhu, Jesus Navarro, Dawn Song, Bo Li, Jacob Steinhardt},
		Subject={ML Safety, Text-Based Games},
		Keywords={ML safety, text-based games, reinforcement learning, transformers, value learning, safe exploration, artificial conscience}
	}
}

\title{What Would Jiminy Cricket Do?\\
Towards Agents That Behave Morally\\Supplementary Material}

\makeatletter
\newcommand{\printfnsymbol}[1]{%
  \textsuperscript{\@fnsymbol{#1}}%
}

\author{
Dan Hendrycks\thanks{Equal Contribution.}\\\hspace{0.7mm}UC Berkeley \And Mantas Mazeika\printfnsymbol{1}\\UIUC \And Andy Zou\\UC Berkeley \And Sahil Patel\\UC Berkeley \AND Christine Zhu\\UC Berkeley \And Jesus Navarro\\UC Berkeley \And Dawn Song\\UC Berkeley \And Bo Li\\UIUC \And Jacob Steinhardt\\UC Berkeley\AND
}

\usepackage{arydshln}

\newcommand{\reviewer}[3]{
	\expandafter\newcommand\csname #1\endcsname[1]{
		\textcolor{#3}{[#2: ##1]}
	}
}
\definecolor{neonpurple}{rgb}{0.3,0,1}
\reviewer{dan}{Dan}{neonpurple}

\begin{document}

\maketitle

\appendix
\input{sections/8-appendix}

\bibliography{main}
\bibliographystyle{plainnat}

\end{document}
